# Supplementary material for: A Comprehensive Analysis of Weakly-Supervised Semantic Segmentation in Different Image Domains
Source: arXiv:1912.11186 ancillary file (2020-10-17)
Supplement: Supplementary file 1 [file ijcv_supplementary.pdf]

# Supplementary Materials for A Comprehensive Analysis of Weakly-Supervised Semantic Segmentation in Different Image Domains

Lyndon Chan · Mahdi S. Hosseini · Konstantinos N. Plataniotis

Received: date / Accepted: date

## 1 Introduction

In the supplementary material, we explain the implementation of the training and tuning procedures used for SEC, DSRG, IRNet, and HistoSegNet and include additional information that will be useful to researchers seeking to replicate the results in the main paper. The supplementary material will be divided as follows.

The first five sections will explain the decisions made behind the training and tuning of the classification CNNs, baseline Grad-CAMs, SEC, DSRG, IRNet, and HistoSegNet:

- Section 2 lists the settings used to train the classification CNNs (VGG16 and X1.7/M7) and provides the training progress plots to show how training converges over time. Weight initialization is conducted with both ImageNet pre-trained weights and with random initialization to show the effect of using pre-trained weight initialization on training.
- Section 3 explains how the baseline Grad-CAM segmentations were generated from the pre-trained classification CNNs.
- Section 4 explains the training setup for SEC and DSRG and how the dense CRF settings were selected, as well as providing the training progress plots to show how training converges over time.
- Section 5 explains the training setup for IRNet and how the dense CRF settings were selected, as well as the preliminary performances during the coordinate descent tuning strategy for each dataset (also described in further detail).
- Section 6 explains the setup for HistoSegNet and how the dense CRF settings were selected.

The final three sections will provide more detailed performance evaluation results and quantitative data relevant to the performance evaluation section (i.e. Section 5) and analysis section (i.e. Section 6) of the main paper:

- Section 7 provides complete per-class segmentation performances in each of the five datasets (including ADP-morph, ADP-func, DeepGlobe, and DeepGlobe (balanced)) evaluated (relevant to Section 5 of the main paper).
- Section 8 provides complete per-class ground-truth instance counts for each of the four evaluation datasets (relevant to Section 6.2 of the main paper).
- Section 9 provides complete ablative study results (with both VGG16 and X1.7) on the effect of seed thresholding levels on SEC and DSRG segmentation performance (relevant to Section 6.2 of the main paper).

## 2 Classification CNN Training

### 2.1 Setup

We selected VGG16 and X1.7/M7 as the classification CNNs to evaluate WSSS in this study, for reasons already explained in the main paper. Network weights were initialized for both VGG16 and X1.7/M7 from the default Keras VGG16 which was already pre-trained on ImageNet. The convolutional layers of X1.7/M7 consists of the first three of five blocks from VGG16, so weights were extracted from the first three blocks only. Note that batch normalization layers were used in VGG16 for VOC2012 and DeepGlobe but not for ADP because these improved training substantially in our experiments. Batch normalization is used in X1.7/M7 for all datasets.

### 2.2 Training Settings

In Table 1, the settings used to train the classification CNNs are listed under four categories. It was decided to resize the images to a square size due to computing and memory constraints. Although this technique was omitted by IRNet, it was used for the original implementations of SEC, DSRG, and HistoSegNet. Image normalization was initially conducted using the dataset intensity mean and standard deviation for ADP and VOC2012 but dropped for DeepGlobe when it turned out to be of little benefit. A more diverse image augmentation strategy is pursued for VOC2012 (i.e. random translation, rotation, zoom, and flip) compared to the simple flipping used for ADP and DeepGlobe because we noted that most objects were situated in the middle of the image in VOC2012 and hence were unlikely to be occluded by vigorous transforms; however, many small segments were located at the image edges in ADP and DeepGlobe, so less vigorous augmentation was used. Cyclical learning rate (CLR) was used instead of a stepwise-decay learning rate schedule because training with CLR tended to converge in fewer epochs and to a higher final accuracy. We experimentally found that the chosen CLR policy worked well for all datasets. The binary cross entropy loss was also weighted for each class by the inverse class frequency in order to prioritize learning in the less common classes, which is especially problematic for imbalanced datasets such as ADP.

| Dataset                   | ADP                                   | VOC2012                       | DeepGlobe       |
|---------------------------|---------------------------------------|-------------------------------|-----------------|
| Image pre-processing      |                                       |                               |                 |
| Image resizing            | To 321x321 (VGG16), 224x224 (X1.7/M7) |                               |                 |
| Image normalization       | $\frac{x-193.09203}{56.4501381}$      | $\frac{x-[104,117,123]}{255}$ | $\frac{x}{255}$ |
| Image augmentation        |                                       |                               |                 |
| Height shift range (%)    | 0                                     | 10                            | 0               |
| Width shift range (%)     | 0                                     | 10                            | 0               |
| Rotation range (degrees)  | 0                                     | 30                            | 0               |
| Zoom range (%)            | 0                                     | 20                            | 0               |
| Horizontal flip           |                                       | TRUE                          |                 |
| Vertical flip             | TRUE                                  | FALSE                         | TRUE            |
| Fill mode                 | None                                  | Reflective                    | None            |
| Learning rate             |                                       |                               |                 |
| CLR policy                |                                       | Triangular                    |                 |
| CLR base learning rate    |                                       | 1.00E-03                      |                 |
| CLR maximum learning rate |                                       | 2.00E-02                      |                 |
| CLR steps per cycle       |                                       | 4                             |                 |
| Learning rate drop step   |                                       | 20                            |                 |
| Learning rate drop rate   |                                       | 0.5                           |                 |
| Other                     |                                       |                               |                 |
| Momentum                  |                                       | 0.9                           |                 |
| Epochs                    |                                       | 80                            |                 |
| Batch size                | 16                                    | 8                             | 8               |
| Class weighting           |                                       | Inverse frequency             |                 |

Table 1: Training settings for classification CNN: (1) image pre-processing, (2) image augmentation, (3) learning rate, and (4) other. CLR stands for ‘‘Cyclical Learning Rate’’

### 2.3 Atlas of Digital Pathology

In Figure 1, training details for VGG16 on ADP are shown, both with and without pre-trained weight initialization. Training details for X1.7 were not shown for the sake of simplicity. Although the pre-trained weights were originally trained on ImageNet, which is a natural scene image dataset, it is clear that using these weights causes better training performance on a histopathology dataset such as ADP compared to random initialization. Using pre-trained weight initialization appears to make no difference on how fast training converges, although the difference in final accuracy is significant - using pre-trained weights confers a 2-3% advantage.

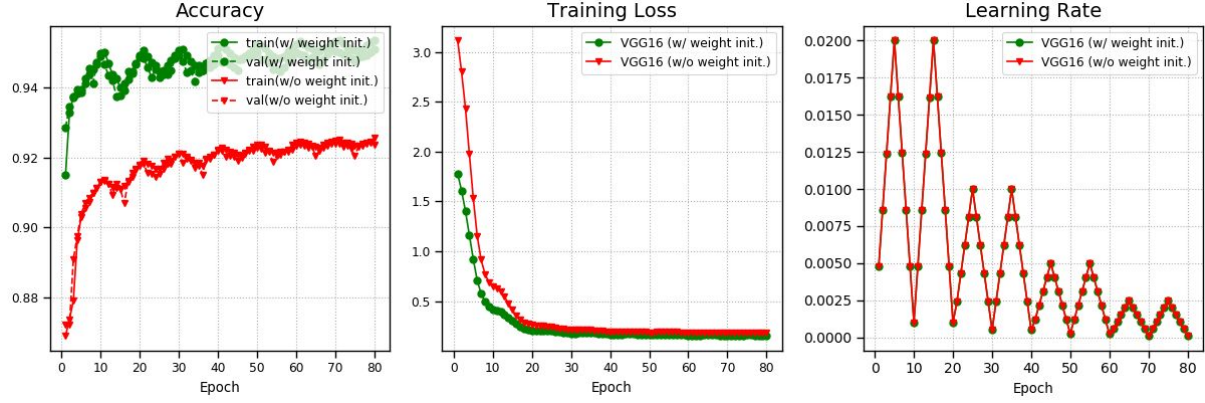

Fig. 1: Training details for VGG16 on ADP, with and without pre-trained weight initialization: (a) accuracy, (b) training loss, and (c) learning rate. Note that vertical scales may not begin at zero.

### 2.4 PASCAL VOC 2012

In Figure 2, training details for VGG16 on VOC2012 are shown, both with and without pre-trained weight initialization. As the pre-trained weights were originally trained on ImageNet, which is also a natural scene image dataset, it is not surprising that using these weights causes better training performance on VOC2012 compared to random initialization. Again, using pre-trained weight initialization appears to make no difference on how fast training converges, although the difference in final accuracy is significant - using pre-trained weights confers an approximately 2% improvement.

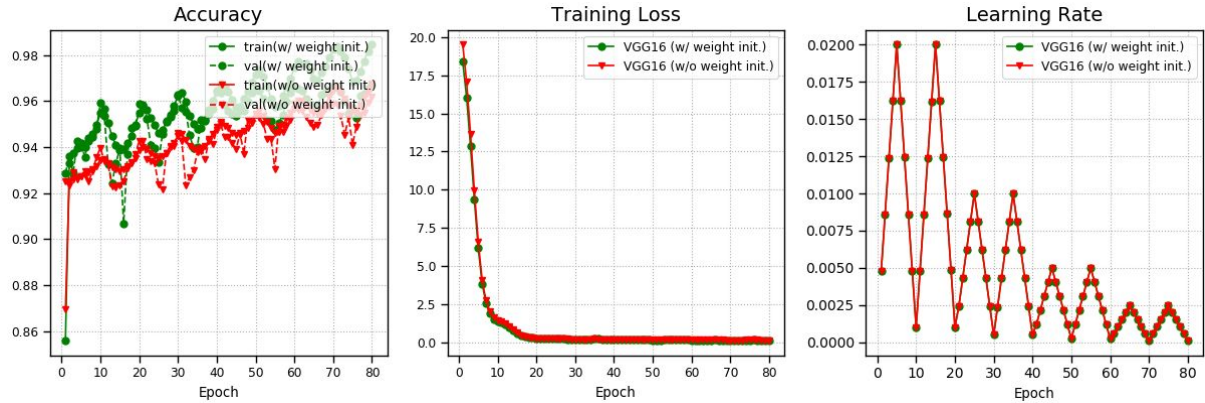

Fig. 2: Training details for VGG16 on VOC2012, with and without pre-trained weight initialization: (a) accuracy, (b) training loss, and (c) learning rate. Note that vertical scales may not begin at zero.

## 2.5 DeepGlobe

In Figure 3, training details for VGG16 on DeepGlobe (without balancing) are shown, both with and without pre-trained weight initialization. Although the pre-trained weights were originally trained on ImageNet, which is a natural scene image dataset, it is clear that using these weights causes better training performance on a satellite image dataset such as DeepGlobe compared to random initialization. In this case, using pre-trained weight initialization appears to make training converge later, although the final accuracy is consistently higher than using random initialization by 5-10%.

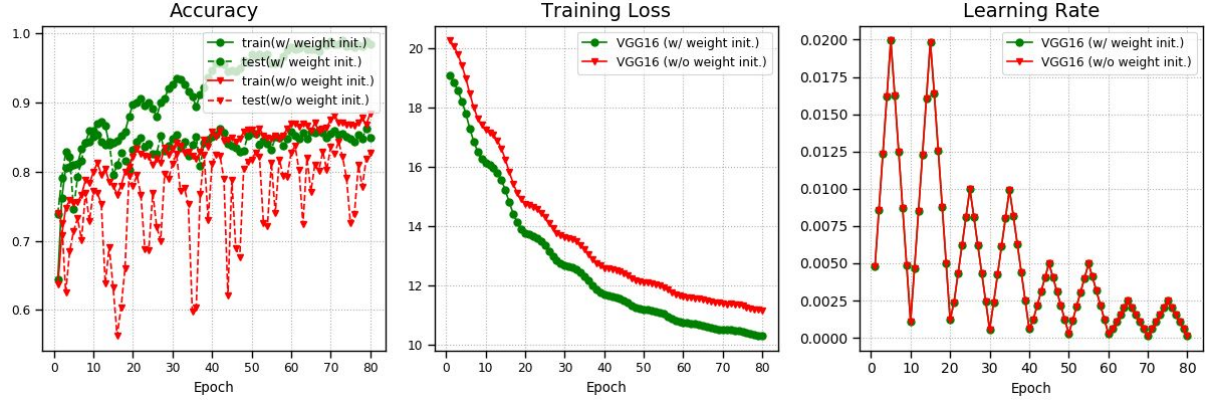

Fig. 3: Training details for VGG16 on DeepGlobe (75% train-25% test split), with and without pre-trained weight initialization: (a) accuracy, (b) training loss, and (c) learning rate. Note that vertical scales may not begin at zero.

## 3 Grad-CAM Baseline

Grad-CAM segmentations were generated using the trained VGG16 and X1.7/M7 classification CNNs to provide the baseline performance. This was done for several reasons: (1) CAM (of which Grad-CAM is a generalized method) was one of the pioneering methods to predict pixel labels when given only image labels for training, and (2) no additional training is required. In order for a WSSS method to be considered feasible, it should at least out-perform Grad-CAM. First, class confidence thresholds were determined for each class at the point in the ROC curve where sensitivity was closest to specificity (the confidence thresholds were clipped to be at least  $\frac{1}{3}$ ). The baseline segmentations were produced by first predicting the Grad-CAMs for each class deemed to be present in a given image; then, the most confident class was taken at each pixel (activation values below 0.15 were considered background, following the optimized settings used by IRNet) and the subsequent segmentation map was upsampled back to the original image size using bilinear interpolation.

## 4 SEC and DSRG Training

### 4.1 Setup

For SEC and DSRG, a simple stepwise decay learning rate schedule was used to train their FCN models, starting at 0.0001 and 0.5 decay every 4 epochs, and training for 16 epochs in total - these were the optimal learning settings used by the TensorFlow code implementations. SEC uses the DeepLabv1 (or DeepLab-LargeFOV) FCN architecture, while DSRG uses the DeepLabv2 (or DeepLab-ASPP) architecture; both initialize their weights using pre-trained weights on ImageNet. DeepLabv2 is a newer architecture with better fully-supervised semantic segmentation performance on the VOC2012 dataset, although it contains 2.79 times the parameters as DeepLabv1 and may not be as suitable for datasets with fewer training images.

Following our own experimentation (as detailed in Section 6.2 of the main paper), we decided to threshold the weak cues at the point where seed coverage reached just under 50%. The same overlapping strategy was used for all datasets: where thresholded activation maps overlapped, the class with the smaller thresholded seed would take precedence. For ADP, this condition had to be met for both the morphological and functional seeds, which was fulfilled when the threshold was set at 90%. For VOC2012, this condition was met at a threshold level of 20%. For DeepGlobe, the optimized threshold was 30% (except for M7 in the unbalanced configuratino, where 40% was optimal).

### 4.2 Dense CRF Settings

The dense CRF settings used to train and evaluate SEC are presented in Tables 2 and 3 respectively. For DSRG, the dense CRF settings are identical for all datasets and are presented together for training and evaluation in Table 4. Our preliminary experiments revealed that utilizing the optimized dense CRF settings provided in the original SEC and DSRG implementations were optimal for training all datasets. For evaluation, the original settings from SEC and DSRG were also found to be optimal for all datasets except for ADP, where we used the optimized settings from HistoSegNet instead.

|              | ADP-morph | ADP-func | VOC2012 | DeepGlobe |
|--------------|-----------|----------|---------|-----------|
| gauss_sxy    | 3 / 12    | 3 / 12   | 3 / 12  | 3 / 12    |
| gauss_compat | 3         | 3        | 3       | 3         |
| bilat_sxy    | 80 / 12   | 80 / 12  | 80 / 12 | 80 / 12   |
| bilat_srgb   | 13        | 13       | 13      | 13        |
| bilat_compat | 10        | 10       | 10      | 10        |
| n_infer      | 5         | 5        | 5       | 5         |

Table 2: Dense CRF settings used to train SEC, for ADP-morph, ADP-func, VOC2012, and DeepGlobe.

|              | ADP-morph | ADP-func | VOC2012 | DeepGlobe |
|--------------|-----------|----------|---------|-----------|
| gauss_sxy    | 1         | 3        | 3       | 3         |
| gauss_compat | 20        | 40       | 3       | 3         |
| bilat_sxy    | 10        | 10       | 80      | 80        |
| bilat_srgb   | 40        | 4        | 13      | 13        |
| bilat_compat | 50        | 25       | 10      | 10        |
| n_infer      | 5         | 5        | 10      | 10        |

Table 3: Dense CRF settings used to evaluate SEC, for ADP-morph, ADP-func, VOC2012, and DeepGlobe.

|              | Training | Evaluation |
|--------------|----------|------------|
| gauss_sxy    | 3 / 12   | 3          |
| gauss_compat | 3        | 3          |
| bilat_sxy    | 80 / 12  | 80         |
| bilat_srgb   | 13       | 13         |
| bilat_compat | 10       | 10         |
| n_infer      | 5        | 5          |

Table 4: Dense CRF settings used to train and evaluate DSRG, for ADP-morph, ADP-func, VOC2012, and DeepGlobe.

## 4.3 ADP-morph

SEC.

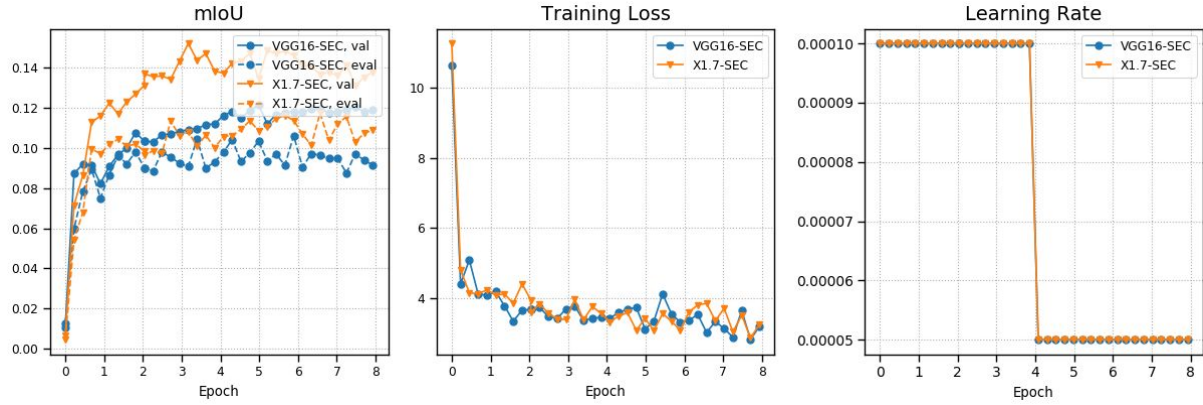

Fig. 4: Training details for SEC on ADP-morph: (a) mean intersection-over-union, (b) training loss, and (c) learning rate.

DSRG.

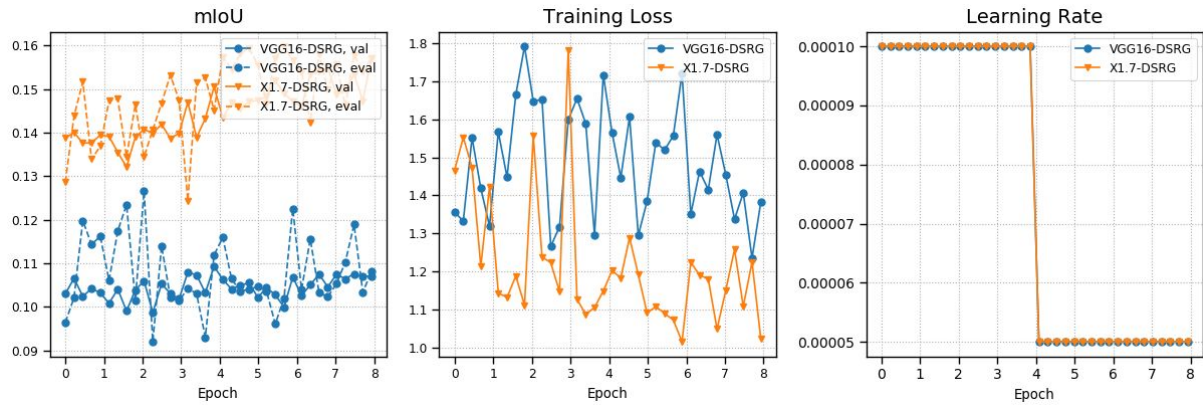

Fig. 5: Training details for DSRG on ADP-morph: (a) mean intersection-over-union, (b) training loss, and (c) learning rate.

## 4.4 ADP-func

SEC.

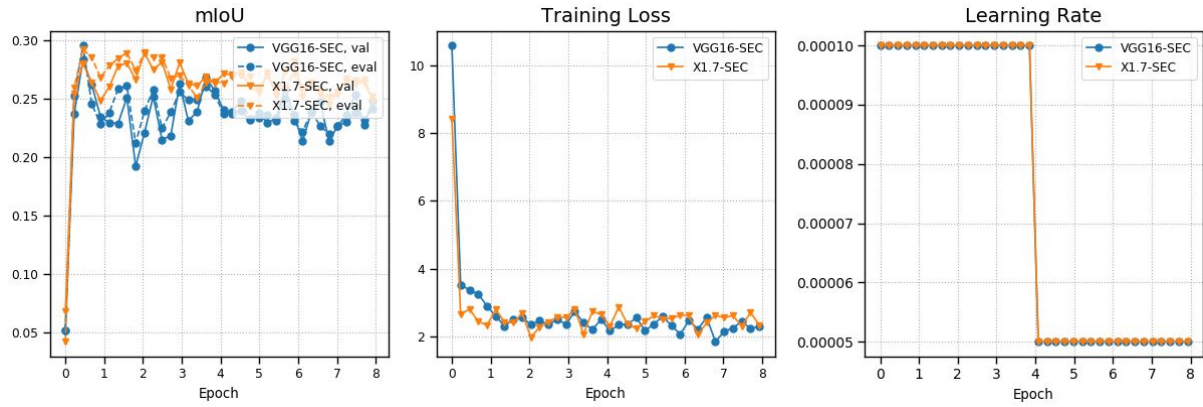

Fig. 6: Training details for SEC on ADP-func: (a) mean intersection-over-union, (b) training loss, and (c) learning rate.

DSRG.

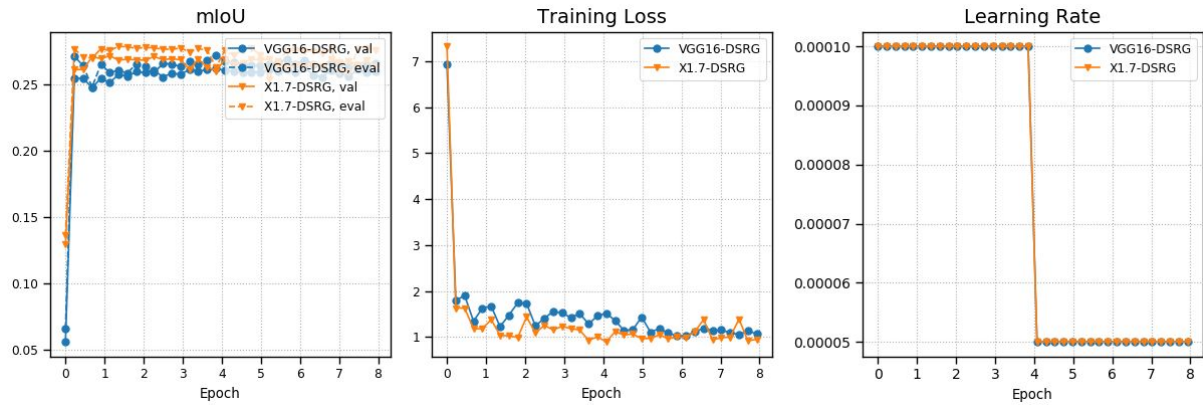

Fig. 7: Training details for DSRG on ADP-func: (a) mean intersection-over-union, (b) training loss, and (c) learning rate.

## 4.5 PASCAL VOC 2012

SEC.

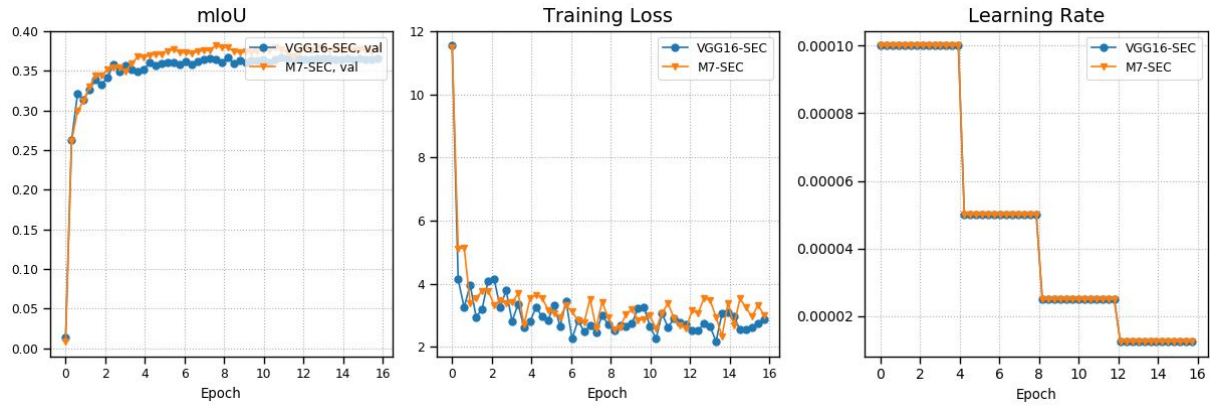

Fig. 8: Training details for SEC on VOC2012: (a) mean intersection-over-union, (b) training loss, and (c) learning rate.

DSRG.

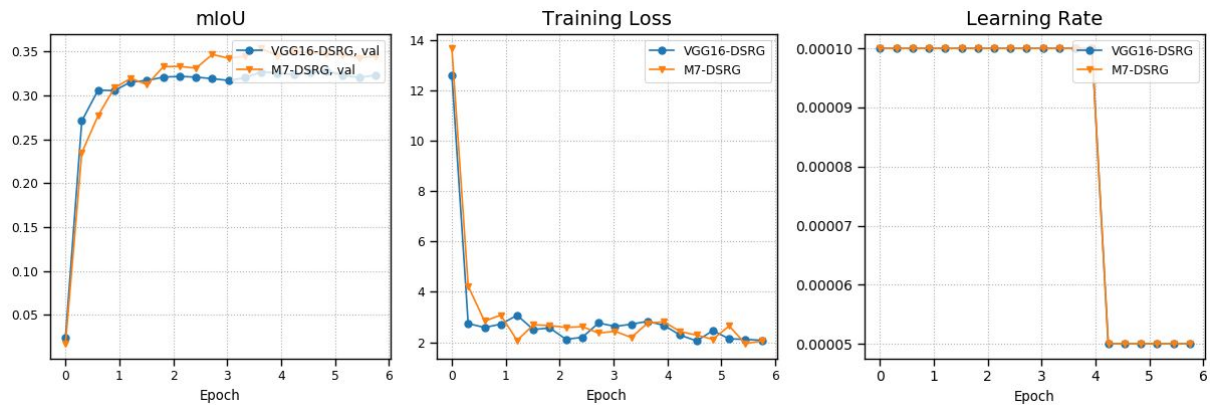

Fig. 9: Training details for DSRG on VOC2012: (a) mean intersection-over-union, (b) training loss, and (c) learning rate.

## 4.6 DeepGlobe

SEC.

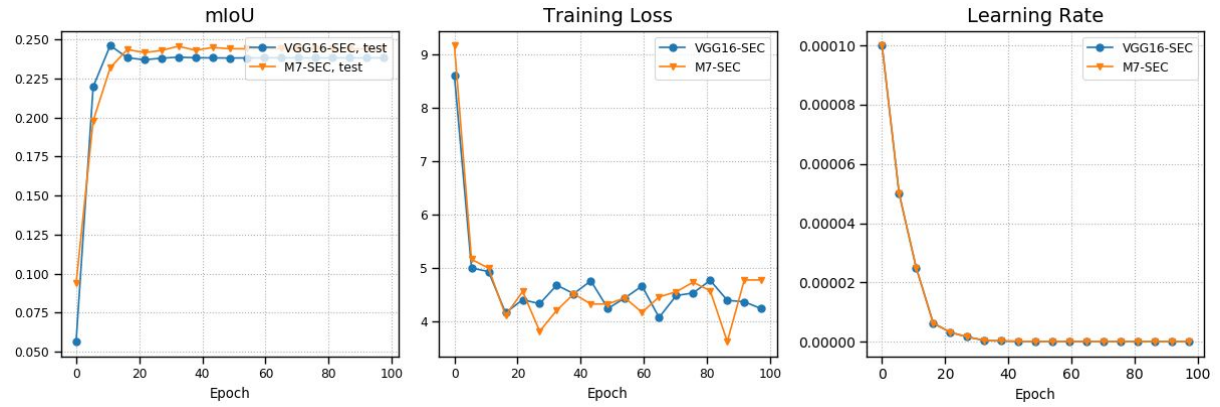

Fig. 10: Training details for SEC on DeepGlobe (75% train-25% test split): (a) mean intersection-over-union, (b) training loss, and (c) learning rate.

DSRG.

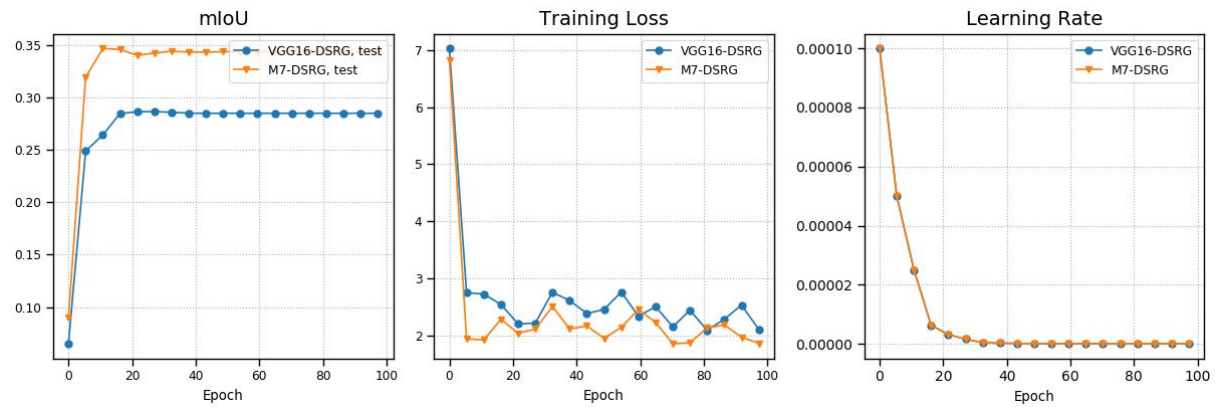

Fig. 11: Training details for DSRG on DeepGlobe (75% train-25% test split): (a) mean intersection-over-union, (b) training loss, and (c) learning rate.

## 4.7 DeepGlobe (balanced)

SEC.

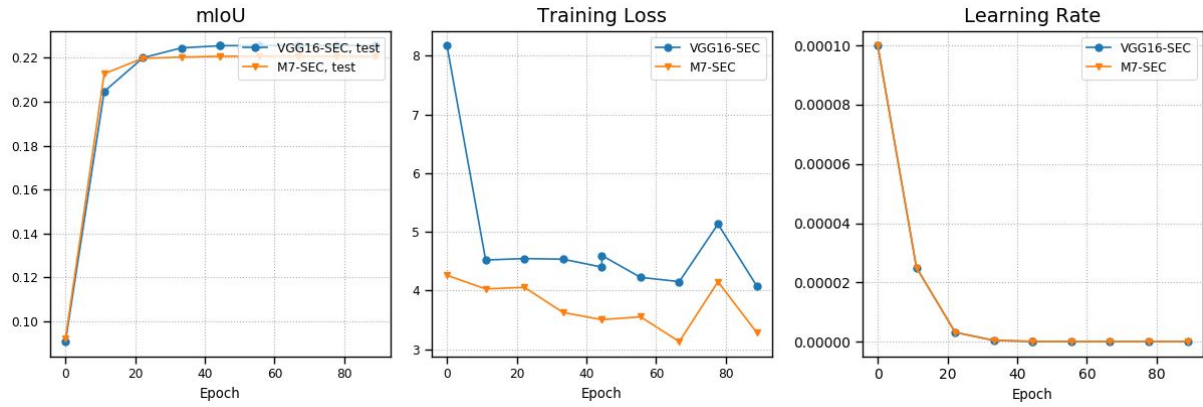

Fig. 12: Training details for SEC on DeepGlobe (37.5% train-25% test split): (a) mean intersection-over-union, (b) training loss, and (c) learning rate.

DSRG.

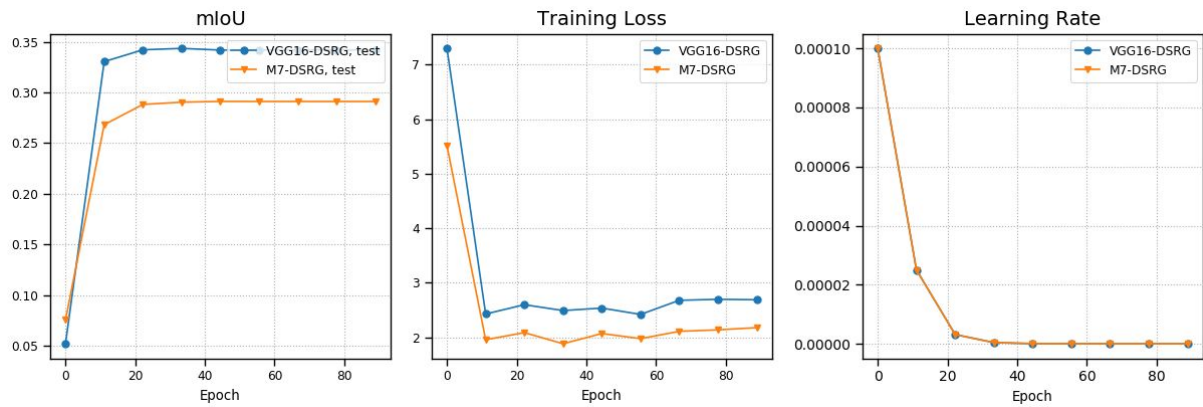

Fig. 13: Training details for DSRG on DeepGlobe (37.5% train-25% test split): (a) mean intersection-over-union, (b) training loss, and (c) learning rate.

## 5 IRNet Tuning

### 5.1 Setup

For IRNet, a constant learning rate of 0.1 and weight decay of 0.0001 were used to train for 3 epochs, following the settings used by the authors. The X1.7/M7 classification CNN uses a Global Max Pooling layer before the Fully-Connected layers, so Grad-CAM was used instead of CAM to generate the pseudo ground-truth segments. Furthermore, architectural modifications had to be made to IRNet to accommodate the alternative backbone networks used. The original implementation of IRNet used ResNet-50 as the backbone network, which has five convolutional layer blocks, each connected to the displacement map and class boundary map branches. VGG16 also has five blocks, so no modifications were needed, but as X1.7/M7 has only three blocks, the branch networks re-connected to these three blocks (e.g. three convolutional layers for three blocks). For ADP, the background activation was generated with the white illumination level and considered as another foreground activation for ADP, while no background activation was considered for DeepGlobe, which lacks such a class.

Our tuning experiments revealed that performance was very sensitive to the value of `conf_fg_thres`, the foreground seeding threshold used to generate pseudo ground-truth segments and the value of `exp_times`, the binary exponent number of steps taken in the random walk to propagate the Grad-CAMs within the class boundary map. Indeed, we found that the default settings for ResNet50 on VOC2012 (i.e. `conf_fg_thres` = 0.3, `exp_times` = 8) produced infeasible segmentation performance for some datasets and networks. To produce reasonably well-tuned performance, we tuned the values of these two hyperparameters using coordinate descent in the two-dimensional hyperparameter space. A starting value was selected for both values and first, the value of `conf_fg_thres` was swept within the range {0.3, 0.5, 0.7}; for each hyperparameter pair, IRNet was trained and evaluated. Once a locally-optimal value of `conf_fg_thres` was found with respect to the mIoU, it was fixed and the value of `exp_times` was varied within the range {1, 2, 3, 4, 5, 6, 7, 8}. The optimal value of `exp_times` was fixed after this sweep.

### 5.2 Dense CRF Settings

In Table 5, the dense CRF settings used for IRNet are presented. IRNet, unlike SEC, DSRG, and HistoSegNet, does not use dense CRF for post-processing, but in order to refine the pseudo ground-truth segmentations before training. Contrary to expectations, the default dense CRF settings (incidentally the same as those for VOC2012 in SEC and DSRG) provided in the original implementation worked well for all datasets.

|                           | ADP-morph | ADP-func | VOC2012 | DeepGlobe |
|---------------------------|-----------|----------|---------|-----------|
| <code>gauss_sxy</code>    | 3 / 12    | 3 / 12   | 3 / 12  | 3 / 12    |
| <code>gauss_compat</code> | 3         | 3        | 3       | 3         |
| <code>bilat_sxy</code>    | 80 / 12   | 80 / 12  | 80 / 2  | 80 / 2    |
| <code>bilat_srgb</code>   | 13        | 13       | 13      | 13        |
| <code>bilat_compat</code> | 10        | 10       | 10      | 10        |
| <code>n_infer</code>      | 5         | 5        | 5       | 5         |

Table 5: Dense CRF settings used to train and evaluate IRNet, for ADP-morph, ADP-func, VOC2012, and DeepGlobe.

### 5.3 Tuning Performance in ADP-morph

VGG16.

| conf_fg_thres | exp_times | mIoU, evaluation |
|---------------|-----------|------------------|
| 0.3           | 1         | 0.148012         |
| 0.5           | 1         | 0.149376         |
| 0.7           | 1         | 0.148132         |
| 0.5           | 2         | 0.150680         |
| 0.5           | 3         | 0.149824         |
| 0.5           | 4         | 0.149000         |
| 0.5           | 5         | 0.150611         |
| 0.5           | 6         | 0.150571         |
| 0.5           | 7         | 0.149717         |
| 0.5           | 8         | 0.144124         |

Table 6: Segmentation performance (mIoU) of VGG16-IRNet on the evaluation set of ADP-morph, for different hyperparameters during coordinate descent tuning. The optimized setting and segmentation performance is highlighted and bolded.

X1.7.

| conf_fg_thres | exp_times | mIoU, evaluation |
|---------------|-----------|------------------|
| 0.3           | 1         | 0.214437         |
| 0.5           | 1         | 0.214502         |
| 0.7           | 1         | 0.213264         |
| 0.5           | 2         | 0.213677         |
| 0.5           | 3         | 0.210566         |
| 0.5           | 4         | 0.205075         |
| 0.5           | 5         | 0.197615         |
| 0.5           | 6         | 0.188356         |
| 0.5           | 7         | 0.175045         |
| 0.5           | 8         | 0.158171         |

Table 7: Segmentation performance (mIoU) of X1.7-IRNet on the evaluation set of ADP-morph, for different hyperparameters during coordinate descent tuning. The optimized setting and segmentation performance is highlighted and bolded.

### 5.4 Tuning Performance in ADP-func

VGG16.

| conf_fg_thres | exp_times | mIoU, evaluation |
|---------------|-----------|------------------|
| 0.3           | 1         | 0.341411         |
| 0.5           | 1         | 0.347717         |
| 0.7           | 1         | 0.348986         |
| 0.7           | 2         | 0.349347         |
| 0.7           | 3         | 0.350160         |
| 0.7           | 4         | 0.350049         |
| 0.7           | 5         | 0.348615         |
| 0.7           | 6         | 0.347958         |
| 0.7           | 7         | 0.346210         |
| 0.7           | 8         | 0.346636         |

Table 8: Segmentation performance (mIoU) of VGG16-IRNet on the evaluation set of ADP-func, for different hyperparameters during coordinate descent tuning. The optimized setting and segmentation performance is highlighted and bolded.

X1.7.

| conf_fg_thres | exp_times | mIoU, evaluation |
|---------------|-----------|------------------|
| 0.3           | 1         | <b>0.347295</b>  |
| 0.5           | 1         | 0.346656         |
| 0.7           | 1         | 0.325624         |
| 0.3           | 2         | 0.340079         |
| 0.3           | 3         | 0.328658         |
| 0.3           | 4         | 0.314360         |
| 0.3           | 5         | 0.296854         |
| 0.3           | 6         | 0.279998         |
| 0.3           | 7         | 0.272685         |
| 0.3           | 8         | 0.262628         |

Table 9: Segmentation performance (mIoU) of X1.7-IRNet on the evaluation set of ADP-func, for different hyperparameters during coordinate descent tuning. The optimized setting and segmentation performance is highlighted and bolded.

## 5.5 Tuning Performance in VOC2012

VGG16.

| conf_fg_thres | exp_times | mIoU, val       |
|---------------|-----------|-----------------|
| 0.3           | 8         | 0.307114        |
| 0.5           | 8         | <b>0.311982</b> |
| 0.7           | 8         | 0.286190        |
| 0.7           | 8         | 0.286190        |
| 0.5           | 1         | 0.253483        |
| 0.5           | 2         | 0.259558        |
| 0.5           | 3         | 0.266412        |
| 0.5           | 4         | 0.274373        |
| 0.5           | 5         | 0.283039        |
| 0.5           | 6         | 0.293418        |
| 0.5           | 7         | 0.303206        |

Table 10: Segmentation performance (mIoU) of VGG16-IRNet on the val set of VOC2012, for different hyperparameters during coordinate descent tuning. The optimized setting and segmentation performance is highlighted and bolded.

M7.

| conf_fg_thres | exp_times | mIoU, val       |
|---------------|-----------|-----------------|
| 0.3           | 3         | 0.176611        |
| 0.5           | 3         | 0.175681        |
| 0.7           | 3         | <b>0.178440</b> |
| 0.7           | 1         | 0.162913        |
| 0.7           | 2         | 0.172872        |
| 0.7           | 4         | 0.177133        |
| 0.7           | 5         | 0.167537        |
| 0.7           | 6         | 0.152674        |
| 0.7           | 7         | 0.138186        |
| 0.7           | 8         | 0.128527        |

Table 11: Segmentation performance (mIoU) of M7-IRNet on the val set of VOC2012, for different hyperparameters during coordinate descent tuning. The optimized setting and segmentation performance is highlighted and bolded.

## 5.6 Tuning Performance in DeepGlobe

VGG16.

| conf_fg_thres | exp_times | mIoU, test      |
|---------------|-----------|-----------------|
| 0.3           | 1         | 0.284791        |
| 0.5           | 1         | 0.285757        |
| 0.7           | 1         | 0.281973        |
| 0.5           | 2         | 0.288594        |
| 0.5           | 3         | 0.291730        |
| 0.5           | 4         | <b>0.294054</b> |
| 0.5           | 5         | 0.293986        |
| 0.5           | 6         | 0.292763        |
| 0.5           | 7         | 0.290560        |
| 0.5           | 8         | 0.286846        |

Table 12: Segmentation performance (mIoU) of VGG16-IRNet on the evaluation set of DeepGlobe, for different hyperparameters during coordinate descent tuning. The optimized setting and segmentation performance is highlighted and bolded.

M7.

| conf_fg_thres | exp_times | mIoU, test      |
|---------------|-----------|-----------------|
| 0.3           | 1         | 0.215501        |
| 0.5           | 1         | 0.218488        |
| 0.7           | 1         | 0.216724        |
| 0.5           | 2         | 0.221155        |
| 0.5           | 3         | 0.224958        |
| 0.5           | 4         | 0.229574        |
| 0.5           | 5         | 0.234198        |
| 0.5           | 6         | 0.239160        |
| 0.5           | 7         | 0.243815        |
| 0.5           | 8         | <b>0.246195</b> |

Table 13: Segmentation performance (mIoU) of M7-IRNet on the evaluation set of DeepGlobe, for different hyperparameters during coordinate descent tuning. The optimized setting and segmentation performance is highlighted and bolded.

## 5.7 Tuning Performance in DeepGlobe (balanced)

VGG16.

| conf_fg_thres | exp_times | mIoU, test      |
|---------------|-----------|-----------------|
| 0.3           | 1         | 0.271805        |
| 0.4           | 1         | 0.272806        |
| 0.5           | 1         | 0.271294        |
| 0.6           | 1         | 0.272242        |
| 0.7           | 1         | 0.270426        |
| 0.4           | 2         | 0.275278        |
| 0.4           | 3         | 0.279041        |
| 0.4           | 4         | 0.283483        |
| 0.4           | 5         | 0.286980        |
| 0.4           | 6         | 0.291060        |
| 0.4           | 7         | <b>0.292068</b> |
| 0.4           | 8         | 0.291668        |

Table 14: Segmentation performance (mIoU) of VGG16-IRNet on the evaluation set of DeepGlobe (balanced), for different hyperparameters during coordinate descent tuning. The optimized setting and segmentation performance is highlighted and bolded.

M7.

| conf_fg_thres | exp_times | mIoU, test      |
|---------------|-----------|-----------------|
| 0.3           | 1         | 0.201740        |
| 0.4           | 1         | 0.201719        |
| 0.5           | 1         | 0.201585        |
| 0.6           | 1         | 0.201576        |
| 0.7           | 1         | 0.202715        |
| 0.7           | 2         | 0.203869        |
| 0.7           | 3         | 0.205467        |
| 0.7           | 4         | 0.207475        |
| 0.7           | 5         | 0.209721        |
| 0.7           | 6         | 0.211923        |
| <b>0.7</b>    | <b>7</b>  | <b>0.213034</b> |
| 0.7           | 8         | 0.212766        |

Table 15: Segmentation performance (mIoU) of M7-IRNet on the evaluation set of DeepGlobe (balanced), for different hyperparameters during coordinate descent tuning. The optimized setting and segmentation performance is highlighted and bolded.

## 6 HistoSegNet Tuning

### 6.1 Setup

For HistoSegNet, no training is conducted after the classification CNN has been trained. As HistoSegNet was originally developed for ADP, no modifications were necessary. But for VOC2012, the background activation had to be generated apart from the Grad-CAMs directly. As in SEC, DSRG, and IRNet, the background activation in VOC2012 was considered the inverse of the foreground class activations. This was generated similarly to the “other” functional activation in ADP: subtracting the sum of foreground class activations from its maximum value, applying a sigmoid to the resultant activations, and multiplying by a scalar constant (i.e. 0.15). No background class exists in DeepGlobe, so no additional handling was used.

### 6.2 Dense CRF Settings

In Table 16, the dense CRF settings used for HistoSegNet are presented. The only setting to be tuned to adjust the method for a new dataset is to select new dense CRF settings using the validation set where available. For ADP-morph and ADP-func, we used the optimized provided by the original authors. For VOC2012, the optimal training settings for dense CRF used in SEC and DSRG were used, but the spatially-relevant settings (i.e. gauss\_sxy, bilat\_sxy) were multiplied by a factor of 6 to increase the strength of post-processing. Likewise, the spatially-relevant settings were multiplied by a factor of 3. We tried different multiplicative factors but these values produced the best results.

|              | ADP-morph | ADP-func | VOC2012 (VGG16) | VOC2012 (M7) | DeepGlobe |
|--------------|-----------|----------|-----------------|--------------|-----------|
| gauss_sxy    | 1         | 3        | 3 / 2           | 3 / 48       | 3 / 2     |
| gauss_compat | 20        | 40       | 3               | 3            | 3         |
| bilat_sxy    | 10        | 10       | 80 / 2          | 80 / 48      | 80 / 2    |
| bilat_srgb   | 40        | 4        | 13              | 13           | 13        |
| bilat_compat | 50        | 25       | 10              | 10           | 10        |
| n_infer      | 5         | 5        | 10              | 10           | 10        |

Table 16: Dense CRF settings used to train and evaluate HistoSegNet, for ADP-morph, ADP-func, VOC2012, and DeepGlobe.

## 7 Detailed Performance Evaluation Results

In this section, the detailed per-class segmentation results are provided for all four methods using the two classification CNNs, as well as the baseline Grad-CAM performance. See Table 17 for ADP-morph, Table 18 for ADP-func, Table 19 for VOC2012, Table 20 for DeepGlobe, and Table 21 for DeepGlobe (balanced).

### 7.1 ADP-morph

| Class      | VGG16    |      |      |       |             | X1.7     |      |      |       |             |
|------------|----------|------|------|-------|-------------|----------|------|------|-------|-------------|
|            | Grad-CAM | SEC  | DSRG | IRNet | HistoSegNet | Grad-CAM | SEC  | DSRG | IRNet | HistoSegNet |
| Background | 48.8     | 24.1 | 40.0 | 52.4  | 56.3        | 23.2     | 23.0 | 59.0 | 26.5  | 50.9        |
| E.M.S      | 0.6      | 0.4  | 0.0  | 0.6   | 0.0         | 1.7      | 1.7  | 0.0  | 1.7   | 3.8         |
| E.M.U      | 11.6     | 15.6 | 9.6  | 11.9  | 9.3         | 17.9     | 13.1 | 18.3 | 18.9  | 21.9        |
| E.M.O      | 5.4      | 4.3  | 0.0  | 4.9   | 4.6         | 25.1     | 24.1 | 0.0  | 25.2  | 24.8        |
| E.T.S      | 18.3     | 0.0  | 0.0  | 26.2  | 43.2        | 41.9     | 0.1  | 62.7 | 42.8  | 66.0        |
| E.T.U      | 5.2      | 4.1  | 0.0  | 4.6   | 0.9         | 6.5      | 12.9 | 0.0  | 7.1   | 10.6        |
| E.T.O      | 0.0      | 0.0  | 0.0  | 0.0   | 0.0         | 0.0      | 6.1  | 0.0  | 0.0   | 0.0         |
| E.P        | 0.0      | 0.0  | 0.0  | 0.0   | 0.0         | 0.0      | 0.0  | 0.0  | 0.0   | 0.0         |
| C.D.I      | 30.7     | 23.1 | 30.4 | 31.4  | 36.4        | 37.7     | 19.9 | 28.8 | 38.4  | 40.6        |
| C.D.R      | 0.0      | 0.0  | 0.0  | 0.0   | 0.0         | 0.0      | 0.0  | 0.0  | 0.0   | 0.0         |
| C.L        | 13.6     | 9.3  | 34.0 | 14.3  | 23.2        | 30.9     | 22.0 | 32.1 | 31.6  | 34.6        |
| H.E        | 5.9      | 13.2 | 9.3  | 6.2   | 7.8         | 15.8     | 14.5 | 1.6  | 15.7  | 29.0        |
| H.K        | 1.1      | 1.8  | 0.0  | 1.2   | 0.0         | 1.6      | 0.0  | 0.0  | 1.7   | 3.8         |
| H.Y        | 1.9      | 1.5  | 0.0  | 1.8   | 2.2         | 6.3      | 5.6  | 0.0  | 6.2   | 7.2         |
| S.M.C      | 78.7     | 0.0  | 0.7  | 72.9  | 70.6        | 66.0     | 1.3  | 0.0  | 66.0  | 68.0        |
| S.M.S      | 21.6     | 28.9 | 24.2 | 22.7  | 22.1        | 37.7     | 24.6 | 19.2 | 37.8  | 35.1        |
| S.E        | 0.0      | 0.0  | 0.0  | 0.0   | 0.0         | 0.0      | 5.0  | 0.0  | 0.0   | 0.0         |
| S.C.H      | 0.0      | 0.0  | 0.0  | 0.0   | 0.0         | 0.0      | 0.0  | 0.0  | 0.0   | 0.0         |
| S.R        | 19.7     | 1.7  | 0.0  | 34.6  | 0.0         | 58.1     | 30.4 | 71.2 | 58.6  | 80.8        |
| A.W        | 23.0     | 1.2  | 0.0  | 17.4  | 0.0         | 47.8     | 0.0  | 0.0  | 48.0  | 1.8         |
| A.B        | 0.0      | 0.0  | 0.0  | 0.0   | 0.0         | 0.0      | 0.0  | 0.0  | 0.0   | 0.0         |
| A.M        | 3.8      | 3.7  | 0.0  | 3.4   | 0.0         | 0.0      | 0.0  | 0.0  | 0.0   | 0.0         |
| M.M        | 44.2     | 27.7 | 10.8 | 42.7  | 50.0        | 47.0     | 30.3 | 0.0  | 47.8  | 53.1        |
| M.K        | 48.1     | 66.9 | 76.8 | 48.1  | 59.0        | 56.3     | 65.9 | 77.4 | 55.7  | 66.4        |
| N.P        | 36.5     | 15.8 | 23.2 | 38.3  | 82.9        | 30.6     | 10.7 | 84.9 | 29.5  | 77.7        |
| N.R.B      | 14.9     | 17.1 | 14.0 | 15.3  | 0.1         | 15.5     | 13.9 | 0.0  | 15.7  | 11.9        |
| N.R.A      | 0.0      | 0.0  | 0.0  | 0.0   | 0.0         | 53.1     | 0.0  | 0.1  | 54.7  | 70.3        |
| N.G.M      | 0.0      | 0.0  | 0.0  | 0.0   | 0.0         | 0.7      | 0.9  | 0.0  | 0.7   | 0.0         |
| N.G.W      | 0.0      | 0.0  | 0.0  | 0.0   | 0.0         | 0.0      | 0.0  | 0.0  | 0.0   | 0.0         |
| Mean       | 14.9     | 9.0  | 9.4  | 15.5  | 16.2        | 21.4     | 11.2 | 15.7 | 21.7  | 26.2        |

Table 17: Per-Class IoU of evaluated methods on the morphological classes of the ADP-morph (evaluation) set (evaluated methods in beige, best-performing evaluated result in bold).

### 7.2 ADP-func

| Class      | VGG16    |      |      |       |             | X1.7     |      |      |       |             |
|------------|----------|------|------|-------|-------------|----------|------|------|-------|-------------|
|            | Grad-CAM | SEC  | DSRG | IRNet | HistoSegNet | Grad-CAM | SEC  | DSRG | IRNet | HistoSegNet |
| Background | 44.1     | 23.9 | 64.4 | 39.3  | 63.8        | 41.6     | 46.5 | 65.9 | 47.7  | 58.1        |
| Other      | 55.2     | 45.3 | 71.4 | 55.8  | 64.4        | 65.0     | 71.2 | 73.1 | 69.1  | 78.8        |
| G.O        | 48.3     | 17.2 | 0.0  | 43.3  | 51.9        | 34.9     | 3.9  | 0.0  | 33.0  | 59.9        |
| G.N        | 38.5     | 18.4 | 0.0  | 38.7  | 36.4        | 44.1     | 7.8  | 0.0  | 42.2  | 33.0        |
| T          | 4.9      | 4.1  | 0.1  | 4.4   | 4.1         | 4.0      | 0.0  | 0.0  | 2.7   | 10.4        |
| Mean       | 38.2     | 21.8 | 27.2 | 36.3  | 44.1        | 37.9     | 25.9 | 27.8 | 38.9  | 48.0        |

Table 18: Per-Class IoU of evaluated methods on the morphological classes of the ADP-func (evaluation) set (evaluated methods in beige, best-performing evaluated result in bold).

## 7.3 VOC2012

| Class       | VGG16    |      |      |       |             | M7       |      |      |       |             |
|-------------|----------|------|------|-------|-------------|----------|------|------|-------|-------------|
|             | Grad-CAM | SEC  | DSRG | IRNet | HistoSegNet | Grad-CAM | SEC  | DSRG | IRNet | HistoSegNet |
| background  | 64.3     | 66.3 | 55.3 | 70.4  | 70.2        | 58.0     | 69.4 | 63.2 | 49.2  | 63.6        |
| aeroplane   | 23.8     | 19.8 | 13.1 | 28.9  | 28.0        | 18.6     | 36.3 | 19.9 | 19.8  | 20.1        |
| bicycle     | 17.4     | 13.7 | 11.4 | 19.2  | 14.9        | 8.3      | 16.8 | 13.3 | 9.5   | 6.5         |
| bird        | 18.4     | 26.8 | 15.3 | 21.5  | 18.7        | 9.9      | 19.2 | 13.8 | 11.5  | 5.9         |
| boat        | 11.7     | 16.0 | 14.0 | 13.2  | 12.0        | 9.1      | 16.5 | 15.0 | 9.7   | 6.9         |
| bottle      | 18.0     | 37.0 | 32.1 | 20.5  | 12.7        | 7.5      | 34.8 | 35.5 | 8.9   | 3.6         |
| bus         | 36.8     | 58.4 | 56.7 | 42.2  | 36.1        | 20.4     | 55.9 | 58.3 | 29.6  | 7.8         |
| car         | 28.4     | 48.9 | 43.7 | 38.8  | 29.0        | 11.5     | 43.2 | 50.9 | 16.8  | 7.9         |
| cat         | 38.6     | 59.9 | 59.4 | 44.9  | 33.3        | 23.3     | 62.7 | 32.3 | 30.2  | 12.8        |
| chair       | 7.0      | 17.0 | 13.7 | 8.5   | 5.9         | 3.5      | 17.9 | 16.4 | 4.4   | 1.7         |
| cow         | 24.5     | 42.8 | 40.9 | 30.0  | 17.2        | 13.7     | 42.3 | 44.1 | 16.4  | 2.1         |
| diningtable | 21.7     | 38.0 | 28.5 | 25.4  | 18.0        | 11.3     | 28.6 | 10.7 | 15.1  | 1.0         |
| dog         | 33.1     | 54.2 | 28.5 | 39.0  | 29.3        | 13.9     | 59.8 | 44.6 | 21.1  | 11.2        |
| horse       | 27.7     | 35.8 | 29.0 | 32.7  | 24.2        | 11.9     | 36.5 | 34.5 | 14.5  | 4.3         |
| motorbike   | 35.4     | 41.7 | 41.4 | 42.2  | 25.7        | 14.9     | 47.4 | 45.8 | 19.8  | 8.1         |
| person      | 30.4     | 43.3 | 44.9 | 36.7  | 29.8        | 8.5      | 35.0 | 57.4 | 12.6  | 8.7         |
| pottedplant | 16.8     | 20.7 | 20.1 | 18.6  | 15.8        | 9.2      | 22.0 | 27.1 | 10.7  | 4.1         |
| sheep       | 25.7     | 37.8 | 29.9 | 33.0  | 8.9         | 24.0     | 44.0 | 52.1 | 29.6  | 1.8         |
| sofa        | 16.3     | 31.3 | 29.1 | 21.2  | 11.9        | 8.3      | 29.5 | 29.4 | 10.6  | 1.3         |
| train       | 31.4     | 39.0 | 37.9 | 39.1  | 11.4        | 18.3     | 36.9 | 36.0 | 22.6  | 7.4         |
| tvmonitor   | 24.3     | 30.1 | 29.7 | 29.3  | 24.6        | 9.9      | 35.5 | 34.9 | 12.2  | 6.6         |
| mIoU        | 26.3     | 37.1 | 32.1 | 31.2  | 22.7        | 14.9     | 37.6 | 35.0 | 17.8  | 9.2         |

Table 19: Per-Class IoU of evaluated methods on the morphological classes of the VOC2012 (test) set (evaluated methods in beige, best-performing evaluated result in bold).

## 7.4 DeepGlobe (75% train-25% test split)

| Class       | VGG16    |      |      |       |             | M7       |      |      |       |             |
|-------------|----------|------|------|-------|-------------|----------|------|------|-------|-------------|
|             | Grad-CAM | SEC  | DSRG | IRNet | HistoSegNet | Grad-CAM | SEC  | DSRG | IRNet | HistoSegNet |
| urban       | 25.3     | 19.8 | 31.5 | 26.2  | 25.9        | 21.1     | 20.8 | 37.6 | 21.0  | 26.9        |
| agriculture | 52.4     | 38.2 | 63.7 | 53.9  | 19.5        | 38.4     | 34.3 | 60.2 | 46.0  | 42.2        |
| rangeland   | 9.9      | 7.9  | 1.0  | 9.5   | 7.9         | 11.6     | 9.5  | 8.9  | 12.3  | 13.8        |
| forest      | 53.4     | 50.0 | 55.8 | 60.1  | 59.3        | 30.4     | 40.8 | 50.6 | 36.7  | 48.4        |
| water       | 5.4      | 5.5  | 0.9  | 5.7   | 11.8        | 6.7      | 19.6 | 21.0 | 8.6   | 12.2        |
| barren      | 21.9     | 22.7 | 20.2 | 21.0  | 19.8        | 19.3     | 24.1 | 33.3 | 23.1  | 32.7        |
| Mean        | 28.0     | 24.0 | 28.8 | 29.4  | 24.1        | 21.3     | 24.8 | 35.3 | 24.6  | 29.4        |

Table 20: Per-Class IoU of evaluated methods on the morphological classes of the DeepGlobe (evaluation) set (evaluated methods in beige, best-performing evaluated result in bold).

## 7.5 DeepGlobe (37.5% train-25% test split)

| Class       | VGG16    |      |      |       |             | M7       |      |      |       |             |
|-------------|----------|------|------|-------|-------------|----------|------|------|-------|-------------|
|             | Grad-CAM | SEC  | DSRG | IRNet | HistoSegNet | Grad-CAM | SEC  | DSRG | IRNet | HistoSegNet |
| urban       | 22.4     | 18.3 | 29.2 | 27.2  | 26.8        | 12.4     | 16.9 | 33.8 | 12.3  | 21.3        |
| agriculture | 49.7     | 46.3 | 62.2 | 48.6  | 25.6        | 45.5     | 39.6 | 65.0 | 49.6  | 24.3        |
| rangeland   | 11.9     | 0.2  | 0.7  | 11.4  | 10.8        | 10.4     | 5.9  | 3.3  | 9.9   | 10.9        |
| forest      | 47.2     | 46.6 | 60.7 | 49.0  | 64.1        | 46.9     | 46.4 | 51.2 | 39.8  | 57.5        |
| water       | 11.2     | 4.6  | 28.1 | 15.1  | 26.0        | 9.4      | 5.6  | 16.4 | 9.0   | 8.9         |
| barren      | 26.1     | 20.0 | 28.7 | 24.0  | 29.2        | 9.0      | 18.9 | 7.7  | 7.2   | 6.7         |
| Mean        | 28.1     | 22.7 | 34.9 | 29.2  | 30.4        | 22.3     | 22.2 | 29.6 | 21.3  | 21.6        |

Table 21: Per-Class IoU of evaluated methods on the morphological classes of the DeepGlobe (evaluation) set (evaluated methods in beige, best-performing evaluated result in bold).

## 8 Detailed Ground-Truth Instance Statistics

In this section, the detailed per-class number of ground-truth instances in the evaluation sets of all four datasets is provided. The average number of instances per image is calculated as the total number of connected components belonging to a particular class in all ground-truth segmentations in the evaluation set, divided by the number of images belonging to that class. The mean average number of instances is the mean of the per-class number of instances, taken across the classes. See Table 22 for ADP-morph, Table 23 for ADP-func, Table 24 for VOC2012, and Table 25 for DeepGlobe.

## 8.1 ADP-morph.

| Classes    | Average Number of Instances |
|------------|-----------------------------|
| Background | 2.571429                    |
| E.M.S      | 1.454545                    |
| E.M.U      | 6.083333                    |
| E.M.O      | 4.153846                    |
| E.T.S      | 2.500000                    |
| E.T.U      | 1.400000                    |
| E.T.O      | 1.500000                    |
| E.P        | 4.000000                    |
| C.D.I      | 7.235294                    |
| C.D.R      | 2.333333                    |
| C.L        | 6.142857                    |
| H.E        | 7.875000                    |
| H.K        | 9.400000                    |
| H.Y        | 13.266667                   |
| S.M.C      | 2.000000                    |
| S.M.S      | 1.000000                    |
| S.E        | 4.000000                    |
| S.C.H      | 1.000000                    |
| S.R        | 4.000000                    |
| A.W        | 3.500000                    |
| A.B        | 1.000000                    |
| A.M        | 22.000000                   |
| M.M        | 9.846154                    |
| M.K        | 7.000000                    |
| N.P        | 4.857143                    |
| N.R.B      | 9.428571                    |
| N.R.A      | 2.333333                    |
| N.G.M      | 11.750000                   |
| N.G.W      | 9.000000                    |
| Mean       | 5.607983                    |

Table 22: Average number of instances per image in the ground-truth segmentation of the evaluation set of the ADP-morph dataset.

## 8.2 ADP-func.

| Classes    | Average Number of Instances |
|------------|-----------------------------|
| Background | 3.848485                    |
| Other      | 1.520000                    |
| G.O        | 4.950000                    |
| G.N        | 6.200000                    |
| T          | 4.793103                    |
| Mean       | 4.262318                    |

Table 23: Average number of instances per image in the ground-truth segmentation of the evaluation set of the ADP-func dataset.

## 8.3 VOC2012.

| Classes     | Average Number of Instances |
|-------------|-----------------------------|
| background  | 0.711656                    |
| aeroplane   | 2.033333                    |
| bicycle     | 2.949367                    |
| bird        | 1.805825                    |
| boat        | 3.361111                    |
| bottle      | 2.187500                    |
| bus         | 0.472973                    |
| car         | 1.811024                    |
| cat         | 1.084034                    |
| chair       | 1.934959                    |
| cow         | 0.338028                    |
| diningtable | 2.520000                    |
| dog         | 0.921875                    |
| horse       | 0.392405                    |
| motorbike   | 2.078947                    |
| person      | 0.600000                    |
| pottedplant | 2.470588                    |
| sheep       | 2.000000                    |
| sofa        | 2.655556                    |
| train       | 0.738095                    |
| tvmonitor   | 1.621622                    |
| Mean        | 1.651852                    |

Table 24: Average number of instances per image in the ground-truth segmentation of the evaluation set of the VOC2012 dataset.

## 8.4 DeepGlobe.

| Classes     | Average Number of Instances |
|-------------|-----------------------------|
| urban       | 1.444444                    |
| agriculture | 0.670330                    |
| rangeland   | 0.630769                    |
| forest      | 3.500000                    |
| water       | 0.681034                    |
| barren      | 2.000000                    |
| unknown     | 2.800000                    |
| Mean        | 1.675225                    |

Table 25: Average number of instances per image in the ground-truth segmentation of the evaluation set of the DeepGlobe dataset.

## 9 Detailed Seed Threshold Ablative Results

In Figure 14, we provide the complete results of the ablative study on the effect of VGG16 and X1.7 seed thresholding levels on subsequent SEC and DSRG performance in ADP-morph. VGG16 and X1.7 seeds are known to have comparatively low recall on ADP-morph, which is connected to poor segmentation performance in SEC and DSRG (see Section 6.2 in the main paper). One method to increase the seed recall is to simply decrease the seed thresholding level, which also increases the mean seed coverage (as seen in Figure 14a and Figure 14b for VGG16 and X1.7 respectively). However, as seen in Figure 14c and Figure 14d, the mIoU of SEC and DSRG actually peak when the recall is lower and the mean seed coverage is just under 50%.

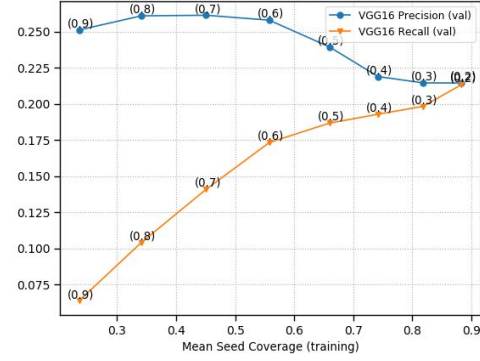

(a) VGG16 Seed Precision and Recall.

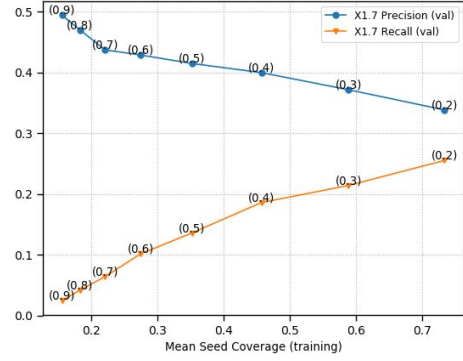

(b) X1.7 Seed Precision and Recall.

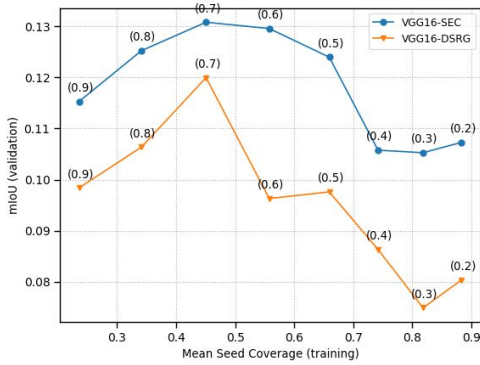

(c) VGG16-SEC and VGG16-DSRG, mIoU.

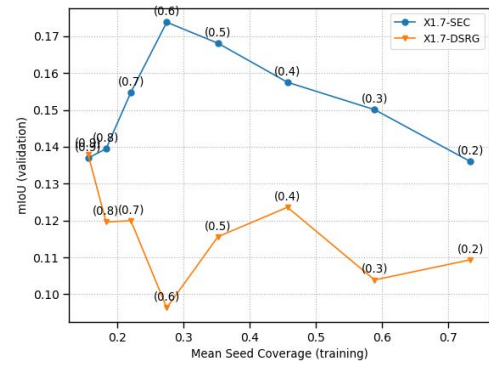

(d) X1.7-SEC and X1.7-DSRG, mIoU.

Fig. 14: Plots of SEC and DSRG segmentation performance (mIoU) (top) and of seed precision and recall (bottom), for different seed threshold levels and seed coverage. Although SEC and DSRG tend to perform better in datasets with high seed recall when seed coverage is set to just under 50%, when seed recall is low for the dataset, increasing the seed coverage to increase the recall (e.g. to 88.3%) actually decreases segmentation mIoU by several percentage points.
